# Supplementary material for: Where Visual Speech Meets Language: VSP-LLM Framework for Efficient and Context-Aware Visual Speech Processing
Source: arXiv:2402.15151 source file (2024-05-14)
Supplement: Supplementary file 1 [file Figure_2_supp.pdf]

## VSR

|                 |               |                                                                                                 |
|-----------------|---------------|-------------------------------------------------------------------------------------------------|
| English<br>(En) | Ground Truth: | it was faulty <b>and</b> most of the time I had to restart it over and over before it worked    |
|                 | Prediction:   | it was <b>failing</b> most of the time I had to restart it over and over before it worked       |
|                 | Ground Truth: | like we evolved on this planet in the context of all the other animals with which we share      |
|                 | Prediction:   | <b>can</b> we evolve on this planet in the context of all the other animals with which we share |

## VST

|                       |               |                                                                                             |
|-----------------------|---------------|---------------------------------------------------------------------------------------------|
| Spanish<br>(En-Es)    | Ground Truth: | tenemos las herramientas pero perdemos la voluntad y el momento <b>colectivo</b>            |
|                       | Prediction:   | tenemos las herramientas pero <b>falta</b> la voluntad <b>colectiva</b> y el momento        |
|                       | Ground Truth: | hay amor y <b>hay</b> amistad y <b>hay</b> protección                                       |
|                       | Prediction:   | hay amor y amistad y protección                                                             |
| Italian<br>(En-It)    | Ground Truth: | utilizza esperienza basata su situazioni simili per imparare a gestire                      |
|                       | Prediction:   | utilizza l'esperienza <b>passata</b> basata su situazioni simili per imparare a <b>fare</b> |
|                       | Ground Truth: | <b>il</b> testo si è sviluppato da questo slash                                             |
|                       | Prediction:   | <b>testando</b> si è sviluppato <b>uno</b> da questo slush                                  |
| French<br>(En-Fr)     | Ground Truth: | comment <b>estce que</b> tu es juste maintenant                                             |
|                       | Prediction:   | comment tu es juste maintenant                                                              |
|                       | Ground Truth: | ce changement devient plus rapide                                                           |
|                       | Prediction:   | ce changement <b>se fait</b> plus <b>rapidement</b>                                         |
| Portuguese<br>(En-Pt) | Ground Truth: | e eu quero fazer o ponto que como membros da sociedade que precisamos                       |
|                       | Prediction:   | e eu quero fazer o ponto <b>de</b> que como membros da sociedade <b>podemos fazer</b>       |
|                       | Ground Truth: | mas a magnitude do problema é quando precisamos aceitar                                     |
|                       | Prediction:   | mas a magnitude do problema é <b>uma vez que</b> precisamos aceitar                         |

| VSR                   |               |                                                                                                 |
|-----------------------|---------------|-------------------------------------------------------------------------------------------------|
| English<br>(En)       | Ground Truth: | it was faulty <b>and</b> most of the time I had to restart it over and over before it worked    |
|                       | Prediction:   | it was <b>failing</b> most of the time I had to restart it over and over before it worked       |
|                       | Ground Truth: | like we evolved on this planet in the context of all the other animals with which we share      |
|                       | Prediction:   | <b>can</b> we evolve on this planet in the context of all the other animals with which we share |
| VST                   |               |                                                                                                 |
| Spanish<br>(En-Es)    | Ground Truth: | tenemos las herramientas pero perdemos la voluntad y el momento <b>colectivo</b>                |
|                       | Prediction:   | tenemos las herramientas pero <b>falta</b> la voluntad <b>colectiva</b> y el momento            |
|                       | Ground Truth: | hay amor y <b>hay</b> amistad y <b>hay</b> protección                                           |
|                       | Prediction:   | hay amor y amistad y protección                                                                 |
| Italian<br>(En-It)    | Ground Truth: | utilizza esperienza basata su situazioni simili per imparare a gestire                          |
|                       | Prediction:   | utilizza l'esperienza <b>passata</b> basata su situazioni simili per imparare a <b>fare</b>     |
|                       | Ground Truth: | <b>il</b> testo si è sviluppato da questo slash                                                 |
|                       | Prediction:   | <b>testando</b> si è sviluppato <b>uno</b> da questo slush                                      |
| French<br>(En-Fr)     | Ground Truth: | comment <b>estce que</b> tu es juste maintenant                                                 |
|                       | Prediction:   | comment tu es juste maintenant                                                                  |
|                       | Ground Truth: | ce changement devient plus rapide                                                               |
|                       | Prediction:   | ce changement <b>se fait</b> plus <b>rapidement</b>                                             |
| Portuguese<br>(En-Pt) | Ground Truth: | e eu quero fazer o ponto que como membros da sociedade que precisamos                           |
|                       | Prediction:   | e eu quero fazer o ponto <b>de</b> que como membros da sociedade <b>podemos fazer</b>           |
|                       | Ground Truth: | mas a magnitude do problema é quando precisamos aceitar                                         |
|                       | Prediction:   | mas a magnitude do problema é <b>uma vez que</b> precisamos aceitar                             |
